# Supplementary material for: Binary Interval Search (BITS): A Scalable Algorithm for Counting Interval Intersections
Source: arXiv:1208.3407 source file (2012-08-17)
Supplement: Supplementary file 1 [file layer-bits-supp.pdf]

# Binary Interval Search (BITS): A Scalable Algorithm for Counting Interval Intersections
*Supplemental Materials*

Ryan M. Layer, Kevin Skadron, Gabriel Robins, Ira M. Hall, and Aaron R. Quinlan

August 16, 2012

## 1 Other BITS algorithms

### 1.1 *Decision problem* (Algorithm 1):

Let $c$ be an accumulator variable that is initialized to zero; then for each $a_i \in A$, accumulate $c = c + \text{ICOUNT}(B_S, B_E, a_i)$. If $c \neq 0$ return *yes*, otherwise return *no*.

### 1.2 *Per-interval counting problem* (Algorithm 2):

Let $C$ be an accumulator array where element $C[i]$ corresponds to the number of intersection for each element in $a_i \in A$. For each $a_i \in A$, set $C[i] = \text{ICOUNT}(B_S, B_E, a_i)$. The total list of counts $C$ is then returned.

### 1.3 *Enumeration problem* (Algorithm 3):

First find the per-interval counting array $C = \text{PERINTERVALCOUNTER}(A, B)$ then the let $R$ be the prefix sum of $C$. The array $R$ is used to track the number of intervals that must be found in each of the subsequent scans. Let $start = 0$ track the number of enumerated intersections. For $i = 1 \ldots |A|$, let

**Algorithm 1:** Intersection decision

**Input**: Database intervals array $B$ and query intervals array $A$
**Output**: *yes* if there is an intersection, otherwise *no*

**Function** $\textsc{Decision}(A, B)$
**begin**
$B_S \leftarrow [b_1.start, \ldots, b_{|B|}.start]$; $B_E \leftarrow [b_1.end, \ldots, b_{|B|}.start]$; $\textsc{Sort}(B_S)$
$\textsc{Sort}(B_E)$
$c \leftarrow 0$
**for** $i \leftarrow 1$ **to** $|A|$ **do**
  $c \leftarrow c + \text{I}\textsc{Count}(B_S, B_E, A[i])$
**if** $c! = 0$ **then**
  **return** yes;
**else**
  **return** no;

**Algorithm 2:** Per-interval intersection counter

**Input**: Database intervals array $B$ and query intervals array $A$
**Output**: Array of intersections counts $C$ where $|C| = |A|$

**Function** $\textsc{PerIntervalCounter}(A, B)$ **begin**
$B_S \leftarrow [b_1.start, \ldots, b_{|B|}.start]$; $B_E \leftarrow [b_1.end, \ldots, b_{|B|}.start]$; $\textsc{Sort}(B_S)$
$\textsc{Sort}(B_E)$
$C \leftarrow [0, \ldots, 0]$
**for** $i \leftarrow 1$ **to** $|A|$ **do**
  $C[i] \leftarrow \text{I}\textsc{Count}(B_S, B_E, A[i])$
**return** $C$

$end = R[i]$ where $end - start$ is the number intervals in $B$ that intersect $a_i$. Let $from = \text{BS}\textsc{earch}(B_S, a_i.end)$ be the initial position of the scan. While $end - start > 0$ some number of intervals in $B$ must be scanned for an intersection with $a_i$. If $a_i$ intersections $b_from$ then let $E[start] =< a_i, b_from >$ and $start = start + 1$. Then let $from = from + 1$. Finally, the total set of intersecting intervals $E$ is returned.

**Algorithm 3:** Intersection enumerator

**Input**: Database intervals array $B$ and query intervals array $A$
**Output**: Array of pair-wise intersections $E$

**Function** ENUMERATOR$(A, B)$ **begin**
  $B_S \leftarrow [b_1.start, \ldots, b_{|B|}.start]$; $B_E \leftarrow [b_1.end, \ldots, b_{|B|}.start]$; SORT$(B_S)$
  SORT$(B_E)$
  $C \leftarrow$ PERINTERVALCOUNTER$(A, B)$
  $R \leftarrow$ PREFIXSUM$(C)$
  $E \leftarrow [<0,0>, \ldots, <0,0>]$
  $start \leftarrow 0$
  **for** $i \leftarrow 1$ **to** $|A|$ **do**
    $end \leftarrow R[i]$
    $from \leftarrow$ BSEARCH$(B_S, A[i].end)$
    **while** $end - start > 0$ **do**
      **if** $A[i]$ *intersects* $B[from]$ **then**
        $E[start] =< A[i], B[from] >$
        $start \leftarrow start + 1$
      $from \leftarrow from - 1$
  **return** $E$

# 2 Sequential Performance Comparison

## 2.1 Counting Comparison

To compare BITS with BEDTOOLS `intersect` and UCSC Genome Browsers ("UCSC") `bedIntersect`, we used internal timers based on the standard C library function `gettimeofday()`. Since BEDTOOLS and BITS perform more sanity checks on input files than `bedIntersection`, wall-time would unfairly penalize BEDTOOLS and BITS. Furthermore, since `bedIntersect` only supports enumeration, the output volume of `bedIntersect` can be much larger than BITS (which reports a single number) and wall-time would unfairly penalize `bedIntersect`. To exclude these differences from the results, we added timers to the source coude of the BEDTOOLS `intersect` and `bedIntersect` source code to ensure that file input was not included in the reported execution time, and all file output commands were commented out.

The modified versions of `bedIntersect` and BEDTOOLS `intersect` are available at:

- http://people.virginia.edu/∼arq5x/files/bits_paper/bedIntersect.c
- http://people.virginia.edu/∼arq5x/files/bits_paper/intersectBed.cpp

## 2.2 Monte Carlo Simulation Comparison

Considering that UCSC `bedIntersect` does not support Monte Carlo (MC) simulations, modifications to the UCSC source were required. MC simulations consist of many rounds of uniformity distributed random interval sets, and `bedIntersect` only supports reading two files from disk and reporting the intersections. One option to add MC simulation support was to first generate random sets using a existing tool (e.g., BEDTools `shuffle` ), then use the unmodified UCSC `bedIntersect` to operate on those random sets. We determined this solution would scale because of the time spent reading and writing these sets. Instead we replaced the function in `bedIntersect` that read interval sets from disk with a function that generates two random interval sets. All subsequent intersection code remained the same. To generate the random interval set, first a random number was generated to determine the chromosome. The likelihood of selecting a particular chromosome is equal the the proportional size of the chromosome in its genome. The next random number represents the staring position of the interval within the chromosome, and the end position is determined by the fixed size given as a command line option. The number of MC rounds is also controlled by a command line parameter.

Since most of the comparisons in an MC simulation are randomly generated, and the number file IO operations is low , we determined that walltime was the best timing mechanism.

The modified version of this code is avaliable at:

- http://people.virginia.edu/∼arq5x/files/bits_paper/randIntersect.c

## 2.3 Computing Environment

Sequential run-times were measured on a 2.0 GHz qua-core Intel Xeon E5504 with 4 MB of cache running Ubuntu Linux version 4.4.3 (kernel version 2.6.32-41). Run-times for CUDA were measured on an NVIDIA Tesla C2050 GPU with 448 1.15 GHz cores, 3 GB of global memory, CUDA driver version 4246739, and CUDA runtime version 4.0. The source code was compiled

using gcc version 4.4.3, and NVIDIA CUDA compilation tools release 4.0, V0.2.1221. Run-times do not include the time required to initialize the GPU.

### 2.4 Files

The NA12878 full-genome and exome-sequencing subsets, and the hg19 exons used to compare the performance of the difference algorithms are available at:

- `http://people.virginia.edu/~arq5x/files/bits_paper/NA12878.exon.tar.gz`
- `http://people.virginia.edu/~arq5x/files/bits_paper/NA12878.full_genome.tar.gz`
- `http://people.virginia.edu/~arq5x/files/bits_paper/exons_hg19.bed.gz`

## 3 Genomic Relationship Experiment Details

All files in this analysis can be downloaded from the UCSC Genome browser site (`http://genome.ucsc.edu/`). ENCODE datasets (i.e., anything beginning with `wgEncode`, are organized under the following URL:
`http://hgdownload.cse.ucsc.edu/goldenPath/hg19/encodeDCC/`

| File Name | Figure Label |
|---|---|
| refseq.hg19.3utr.bed | 3UTR |
| refseq.hg19.5utr.bed | 5UTR |
| aluY.hg19.bed | Aluy |
| 29way_pi.conservation.hg19.bed | Conservation |
| refseq.hg19.downstream.5kb.bed | Downstream |
| cpg-islands.hg19.bed | CPG-islands |
| refseq.hg19.exons.bed | Exons |
| refseq.hg19.introns.bed | Introns |
| L1.hg19.bed | L1 |
| microsatellites.hg19.bed.bed | Microsatellites |
| segdups.hg19.bed | Segdups |
| refseq.hg19.wholegene.bed | Wholegene |
| wgEncodeHaibTfbsGm12878Atf3Pcr1xPkRep1.broadPeak | Atf3 GM12878 |
| wgEncodeHaibTfbsGm12878Atf3Pcr1xPkRep2.broadPeak | Atf3 GM12878 |
| wgEncodeHaibTfbsH1hescAtf3V0416102PkRep1.broadPeak | Atf3 H1-hESC |
| wgEncodeHaibTfbsH1hescAtf3V0416102PkRep2.broadPeak | Atf3 H1-hESC |
| wgEncodeHaibTfbsK562Atf3V0416101PkRep1.broadPeak | Atf3 K562-1 |
| wgEncodeHaibTfbsK562Atf3V0416101PkRep2.broadPeak | Atf3 K562-2 |

| | |
|---|---|
| wgEncodeSydhTfbsGm12878Chd2ab68301IggmusPk.narrowPeak | Chd2 GM12878 |
| wgEncodeSydhTfbsH1hescChd2IggrabPk.narrowPeak | Chd2 H1-hESC |
| wgEncodeSydhTfbsK562Chd2ab68301IggrabPk.narrowPeak | Chd2 K562 |
| wgEncodeOpenChromChipGm12878CmycPk.narrowPeak | Cmyc GM12878 |
| wgEncodeOpenChromChipH1hescCmycPk.narrowPeak | Cmyc H1-hESC |
| wgEncodeOpenChromChipK562CmycPk.narrowPeak | Cmyc K562 |
| wgEncodeBroadChipSeqPeaksGm12878Ctcf.broadPeak | Ctcf GM12878 |
| wgEncodeBroadChipSeqPeaksH1hescCtcf.broadPeak | Ctcf H1-hESC |
| wgEncodeBroadChipSeqPeaksK562Ctcf.broadPeak | Ctcf K562 |
| wgEncodeOpenChromDnaseGm12878Pk.narrowPeak | Dnase GM12878 |
| wgEncodeOpenChromDnaseH1hescPk.narrowPeak | Dnase H1-hESC |
| wgEncodeOpenChromDnaseK562PkV2.narrowPeak | Dnase K562 |
| wgEncodeHaibTfbsGm12878Egr1V0416101PkRep1.broadPeak | Egr1 GM12878-1 |
| wgEncodeHaibTfbsGm12878Egr1V0416101PkRep2.broadPeak | Egr1 GM12878-2 |
| wgEncodeHaibTfbsH1hescEgr1V0416102PkRep1.broadPeak | Egr1 H1-hESC-1 |
| wgEncodeHaibTfbsH1hescEgr1V0416102PkRep2.broadPeak | Egr1 H1-hESC-2 |
| wgEncodeHaibTfbsK562Egr1V0416101PkRep1.broadPeak | Egr1 K562-1 |
| wgEncodeHaibTfbsK562Egr1V0416101PkRep2.broadPeak | Egr1 K562-2 |
| wgEncodeOpenChromFaireGm12878Pk.narrowPeak | FAIRE GM12878 |
| wgEncodeOpenChromFaireH1hescPk.narrowPeak | FAIRE H1-hESC |
| wgEncodeOpenChromFaireK562Pk.narrowPeak | FAIRE K562 |
| wgEncodeHaibTfbsGm12878GabpPcr2xPkRep1.broadPeak | Gabp GM12878-1 |
| wgEncodeHaibTfbsGm12878GabpPcr2xPkRep2.broadPeak | Gabp GM12878-2 |
| wgEncodeHaibTfbsH1hescGabpPcr1xPkRep1.broadPeak | Gabp H1-hESC-1 |
| wgEncodeHaibTfbsH1hescGabpPcr1xPkRep2.broadPeak | Gabp H1-hESC-2 |
| wgEncodeHaibTfbsK562GabpV0416101PkRep1.broadPeak | Gabp K562-1 |
| wgEncodeHaibTfbsK562GabpV0416101PkRep2.broadPeak | Gabp K562-2 |
| wgEncodeBroadChipSeqPeaksGm12878H3k27ac.broadPeak | H3k27ac GM12878 |
| wgEncodeBroadChipSeqPeaksK562H3k27ac.broadPeak | H3k27ac K562 |
| wgEncodeBroadChipSeqPeaksGm12878H3k27me3.broadPeak | H3k27me3 GM12878 |
| wgEncodeBroadChipSeqPeaksH1hescH3k27me3.broadPeak | H3k27me3 H1-hESC |
| wgEncodeBroadChipSeqPeaksK562H3k27me3.broadPeak | H3k27me3 K562 |
| wgEncodeBroadChipSeqPeaksGm12878H3k36me3.broadPeak | H3k36me3 GM12878 |
| wgEncodeBroadChipSeqPeaksH1hescH3k36me3.broadPeak | H3k36me3 H1-hESC |
| wgEncodeBroadChipSeqPeaksK562H3k36me3.broadPeak | H3k36me3 K562 |
| wgEncodeBroadChipSeqPeaksGm12878H3k4me1.broadPeak | H3k4me1 GM12878 |
| wgEncodeBroadChipSeqPeaksH1hescH3k4me1.broadPeak | H3k4me1 H1-hESC |
| wgEncodeBroadChipSeqPeaksK562H3k4me1.broadPeak | H3k4me1 K562 |
| wgEncodeBroadChipSeqPeaksGm12878H3k4me2.broadPeak | H3k4me2 GM12878 |
| wgEncodeBroadChipSeqPeaksH1hescH3k4me2.broadPeak | H3k4me2 H1-hESC |
| wgEncodeBroadChipSeqPeaksK562H3k4me2.broadPeak | H3k4me2 K562 |
| wgEncodeBroadChipSeqPeaksGm12878H3k4me3.broadPeak | H3k4me3 GM12878 |
| wgEncodeBroadChipSeqPeaksH1hescH3k4me3.broadPeak | H3k4me3 H1-hESC |
| wgEncodeBroadChipSeqPeaksK562H3k4me3.broadPeak | H3k4me3 K562 |
| wgEncodeBroadChipSeqPeaksGm12878H3k9ac.broadPeak | H3k9ac GM12878 |

| | |
|---|---|
| wgEncodeBroadChipSeqPeaksH1hescH3k9ac.broadPeak | H3k9ac H1-hESC |
| wgEncodeBroadChipSeqPeaksK562H3k9ac.broadPeak | H3k9ac K562 |
| wgEncodeBroadChipSeqPeaksK562H3k9me1.broadPeak | H3k9me1 K562 |
| wgEncodeBroadChipSeqPeaksGm12878H4k20me1.broadPeak | H4k20me1 GM12878 |
| wgEncodeBroadChipSeqPeaksH1hescH4k20me1.broadPeak | H4k20me1 H1-hESC |
| wgEncodeBroadChipSeqPeaksK562H4k20me1.broadPeak | H4k20me1 K562 |
| wgEncodeSydhTfbsGm12878JundStdPk.narrowPeak | Jund GM12878 |
| wgEncodeSydhTfbsH1hescJundIggrabPk.narrowPeak | Jund H1-hESC |
| wgEncodeSydhTfbsK562JundIggrabPk.narrowPeak | Jund K562 |
| wgEncodeHaibMethyl450Gm12878SitesRep1.methylated.bed | Meth GM12878 |
| wgEncodeHaibMethyl450H1hescSitesRep1.methylated.bed | Meth H1-hESC |
| wgEncodeHaibMethyl450K562SitesRep1.methylated.bed | Meth K562 |
| wgEncodeSydhTfbsGm12878Mxi1IggmusPk.narrowPeak | Mxi1 GM12878 |
| wgEncodeSydhTfbsH1hescMxi1IggrabPk.narrowPeak | Mxi1 H1-hESC |
| wgEncodeSydhTfbsK562Mxi1af4185IggrabPk.narrowPeak | Mxi1 K562 |
| wgEncodeSydhTfbsGm12878Nrf1IggmusPk.narrowPeak | Nrf1 GM12878 |
| wgEncodeSydhTfbsH1hescNrf1IggrabPk.narrowPeak | Nrf1 H1-hESC |
| wgEncodeSydhTfbsK562Nrf1IggrabPk.narrowPeak | Nrf1 K562 |
| wgEncodeHaibTfbsGm12878Pol2Pcr2xPkRep1.broadPeak | Pol2 GM12878-1 |
| wgEncodeHaibTfbsGm12878Pol2Pcr2xPkRep2.broadPeak | Pol2 GM12878-2 |
| wgEncodeOpenChromChipGm12878Pol2Pk.narrowPeak | Pol2 GM12878-3 |
| wgEncodeHaibTfbsH1hescPol2V0416102PkRep1.broadPeak | Pol2 H1-hESC-1 |
| wgEncodeHaibTfbsH1hescPol2V0416102PkRep2.broadPeak | Pol2 H1-hESC-2 |
| wgEncodeOpenChromChipH1hescPol2Pk.narrowPeak | Pol2 H1-hESC-3 |
| wgEncodeHaibTfbsK562Pol2V0416101PkRep1.broadPeak | Pol2 K562-1 |
| wgEncodeHaibTfbsK562Pol2V0416101PkRep2.broadPeak | Pol2 K562-2 |
| wgEncodeOpenChromChipK562Pol2Pk.narrowPeak | Pol2 K562 |
| wgEncodeHaibTfbsGm12878Pol24h8Pcr1xPkRep1.broadPeak | Pol24h8 GM12878-1 |
| wgEncodeHaibTfbsGm12878Pol24h8Pcr1xPkRep2.broadPeak | Pol24h8 GM12878-2 |
| wgEncodeHaibTfbsH1hescPol24h8V0416102PkRep1.broadPeak | Pol24h8 H1-hESC-1 |
| wgEncodeHaibTfbsH1hescPol24h8V0416102PkRep2.broadPeak | Pol24h8 H1-hESC-2 |
| wgEncodeHaibTfbsK562Pol24h8V0416101PkRep1.broadPeak | Pol24h8 K562-1 |
| wgEncodeHaibTfbsK562Pol24h8V0416101PkRep2.broadPeak | Pol24h8 K562-2 |
| wgEncodeBroadChipSeqPeaksK562Pol2b.broadPeak | Pol2b K562 |
| refseq.hg19.promoters.5kb.bed | Promoters |
| wgEncodeHaibTfbsGm12878Rad21V0416101PkRep1.broadPeak | Rad21 GM12878-1 |
| wgEncodeHaibTfbsGm12878Rad21V0416101PkRep2.broadPeak | Rad21 GM12878-2 |
| wgEncodeSydhTfbsGm12878Rad21IggrabPk.narrowPeak | Rad21 GM12878-3 |
| wgEncodeHaibTfbsH1hescRad21V0416102PkRep1.broadPeak | Rad21 H1-hESC-1 |
| wgEncodeHaibTfbsH1hescRad21V0416102PkRep2.broadPeak | Rad21 H1-hESC-2 |
| wgEncodeSydhTfbsH1hescRad21IggrabPk.narrowPeak | Rad21 H1-hESC-3 |
| wgEncodeHaibTfbsK562Rad21V0416102PkRep1.broadPeak | Rad21 K562-1 |
| wgEncodeHaibTfbsK562Rad21V0416102PkRep2.broadPeak | Rad21 K562-2 |
| wgEncodeSydhTfbsK562Rad21StdPk.narrowPeak | Rad21 K562-3 |
| wgEncodeSydhTfbsGm12878Rfx5200401194IggmusPk.narrowPeak | Rfx5 GM12878 |

| | |
|---|---|
| wgEncodeSydhTfbsH1hescRfx5200401194IggrabPk.narrowPeak | Rfx5 H1-hESC |
| wgEncodeSydhTfbsK562Rfx5IggrabPk.narrowPeak | Rfx5 K562 |
| wgEncodeHaibMethyl450Gm12878SitesRep1.semi-methylated.bed | Semi-meth GM12878 |
| wgEncodeHaibMethyl450H1hescSitesRep1.semi-methylated.bed | Semi-meth H1-hESC |
| wgEncodeHaibMethyl450K562SitesRep1.semi-methylated.bed | Semi-meth K562 |
| wgEncodeHaibTfbsGm12878Six5Pcr1xPkRep1.broadPeak | Six5 GM12878-1 |
| wgEncodeHaibTfbsGm12878Six5Pcr1xPkRep2.broadPeak | Six5 GM12878-2 |
| wgEncodeHaibTfbsH1hescSix5Pcr1xPkRep1.broadPeak | Six5 H1-hESC-1 |
| wgEncodeHaibTfbsH1hescSix5Pcr1xPkRep2.broadPeak | Six5 H1-hESC-2 |
| wgEncodeHaibTfbsK562Six5Pcr1xPkRep1.broadPeak | Six5 K562-1 |
| wgEncodeHaibTfbsK562Six5Pcr1xPkRep2.broadPeak | Six5 K562-2 |
| wgEncodeHaibTfbsGm12878Sp1Pcr1xPkRep1.broadPeak | Sp1 GM12878-1 |
| wgEncodeHaibTfbsGm12878Sp1Pcr1xPkRep2.broadPeak | Sp1 GM12878-2 |
| wgEncodeHaibTfbsH1hescSp1Pcr1xPkRep1.broadPeak | Sp1 H1-hESC-1 |
| wgEncodeHaibTfbsH1hescSp1Pcr1xPkRep2.broadPeak | Sp1 H1-hESC-2 |
| wgEncodeHaibTfbsK562Sp1Pcr1xPkRep1.broadPeak | Sp1 K562-1 |
| wgEncodeHaibTfbsK562Sp1Pcr1xPkRep2.broadPeak | Sp1 K562-2 |
| wgEncodeHaibTfbsGm12878SrfV0416101PkRep1.broadPeak | Srf GM12878-1 |
| wgEncodeHaibTfbsGm12878SrfV0416101PkRep2.broadPeak | Srf GM12878-2 |
| wgEncodeHaibTfbsH1hescSrfPcr1xPkRep1.broadPeak | Srf H1-hESC-1 |
| wgEncodeHaibTfbsH1hescSrfPcr1xPkRep2.broadPeak | Srf H1-hESC-2 |
| wgEncodeHaibTfbsK562SrfV0416101PkRep1.broadPeak | Srf K562-1 |
| wgEncodeHaibTfbsK562SrfV0416101PkRep2.broadPeak | Srf K562-2 |
| wgEncodeHaibTfbsGm12878Taf1Pcr1xPkRep1.broadPeak | Taf1 GM12878-1 |
| wgEncodeHaibTfbsGm12878Taf1Pcr1xPkRep2.broadPeak | Taf1 GM12878-2 |
| wgEncodeHaibTfbsH1hescTaf1V0416102PkRep1.broadPeak | Taf1 H1-hESC-1 |
| wgEncodeHaibTfbsH1hescTaf1V0416102PkRep2.broadPeak | Taf1 H1-hESC-2 |
| wgEncodeHaibTfbsK562Taf1V0416101PkRep1.broadPeak | Taf1 K562-1 |
| wgEncodeHaibTfbsK562Taf1V0416101PkRep2.broadPeak | Taf1 K562-2 |
| wgEncodeSydhTfbsGm12878TbpIggmusPk.narrowPeak | Tbp GM12878 |
| wgEncodeSydhTfbsH1hescTbpIggrabPk.narrowPeak | Tbp H1-hESC |
| wgEncodeSydhTfbsK562TbpIggmusPk.narrowPeak | Tbp K562 |
| wgEncodeHaibMethyl450Gm12878SitesRep1.unmethylated.bed | Un-meth GM12878 |
| wgEncodeHaibMethyl450H1hescSitesRep1.unmethylated.bed | Un-meth H1-hESC |
| wgEncodeHaibMethyl450K562SitesRep1.unmethylated.bed | Un-meth K562 |
| wgEncodeHaibTfbsGm12878Usf1Pcr2xPkRep1.broadPeak | Usf1 GM12878-1 |
| wgEncodeHaibTfbsGm12878Usf1Pcr2xPkRep2.broadPeak | Usf1 GM12878-2 |
| wgEncodeHaibTfbsH1hescUsf1Pcr1xPkRep1.broadPeak | Usf1 H1-hESC-1 |
| wgEncodeHaibTfbsH1hescUsf1Pcr1xPkRep2.broadPeak | Usf1 H1-hESC-2 |
| wgEncodeHaibTfbsK562Usf1V0416101PkRep1.broadPeak | Usf1 K562-1 |
| wgEncodeHaibTfbsK562Usf1V0416101PkRep2.broadPeak | Usf1 K562-2 |
| wgEncodeSydhTfbsGm12878Usf2IggmusPk.narrowPeak | Usf2 GM12878 |
| wgEncodeSydhTfbsH1hescUsf2IggrabPk.narrowPeak | Usf2 H1-hESC |
| wgEncodeSydhTfbsK562Usf2IggrabPk.narrowPeak | Usf2 K562 |
| wgEncodeHaibTfbsGm12878Yy1sc281Pcr1xPkRep1.broadPeak | Yy1 GM12878-1 |

| | |
|---|---|
| wgEncodeHaibTfbsGm12878Yy1sc281Pcr1xPkRep2.broadPeak | Yy1 GM12878-2 |
| wgEncodeHaibTfbsH1hescYy1sc281V0416102PkRep1.broadPeak | Yy1 H1-hESC-1 |
| wgEncodeHaibTfbsH1hescYy1sc281V0416102PkRep2.broadPeak | Yy1 H1-hESC-2 |
| wgEncodeHaibTfbsK562Yy1sc281V0416101PkRep1.broadPeak | Yy1 K562-1 |
| wgEncodeHaibTfbsK562Yy1sc281V0416101PkRep2.broadPeak | Yy1 K562-2 |
| wgEncodeSydhTfbsGm12878Znf143166181apStdPk.narrowPeak | Znf143 GM12878 |
| wgEncodeSydhTfbsH1hescZnf143IggrabPk.narrowPeak | Znf143 H1-hESC |
| wgEncodeSydhTfbsK562Znf143IggrabPk.narrowPeak | Znf143 K562 |
